# Supplementary material for: DiffPoint: Single and Multi-view Point Cloud Reconstruction with ViT Based Diffusion Model
Source: arXiv:2402.11241 source file (2024-02-17)
Supplement: Supplementary file 1 [file X_suppl.tex]

\clearpage
\setcounter{page}{1}
\maketitlesupplementary


\section{Experimental Setup}
\label{sec:rationale}
% 
Having the supplementary compiled together with the main paper means that:
% 
\begin{itemize}
\item The supplementary can back-reference sections of the main paper, for example, we can refer to \cref{sec:intro};
\item The main paper can forward reference sub-sections within the supplementary explicitly (e.g. referring to a particular experiment); 
\item When submitted to arXiv, the supplementary will already included at the end of the paper.
\end{itemize}
% 
To split the supplementary pages from the main paper, you can use \href{https://support.apple.com/en-ca/guide/preview/prvw11793/mac#:~:text=Delete%20a%20page%20from%20a,or%20choose%20Edit%20%3E%20Delete).}{Preview (on macOS)}, \href{https://www.adobe.com/acrobat/how-to/delete-pages-from-pdf.html#:~:text=Choose%20%E2%80%9CTools%E2%80%9D%20%3E%20%E2%80%9COrganize,or%20pages%20from%20the%20file.}{Adobe Acrobat} (on all OSs), as well as \href{https://superuser.com/questions/517986/is-it-possible-to-delete-some-pages-of-a-pdf-document}{command line tools}.

\begin{table*}[htbp!]
\centering
\caption{Point based diffusion model comparison for single-view reconstruction on ShapeNet.}
\label{tab:exp_setup}
\scalebox{0.7}{
\begin{tabular}{c| c c c c c c c c c c c c} 
\toprule[2pt]
    {Methods} &Dataset & Bachsize &Optimizer &Learning rate &Weight decay & Sampling steps &$\beta_1$ &$\beta_T$ &embedding dim &depth & number of heads &#Params\\
\midrule[2pt]
\midrule[2pt]
      DiffPoint-S &ShapeNet &128 &AdamW &2e-4 &1e-4 &ShapeNet &ShapeNet &ShapeNet &ShapeNet  &ShapeNet &ShapeNet &ShapeNet\\
      DiffPoint-M &ShapeNet &128 &AdamW &2e-4 &1e-4 &ShapeNet &ShapeNet &ShapeNet  &ShapeNet &ShapeNet &ShapeNet &ShapeNet\\
      DiffPoint-M &OBJAVERSE &128 &AdamW &2e-4 &1e-4 &ShapeNet &ShapeNet &ShapeNet  &ShapeNet &ShapeNet &ShapeNet\\
\bottomrule[2pt]
\end{tabular}}
\end{table*}
